# Supplementary material for: Slicer Networks
Source: arXiv:2401.09833 source file (2024-01-18)
Supplement: Supplementary file 1 [file appendix.tex]

\section{Appendix Section}
Supplementary material goes here.
